# Supplementary material for: Paracosm: A Language and Tool for Testing Autonomous Driving Systems
Source: arXiv:1902.01084 source file (2021-01-15)
Supplement: Supplementary file 1 [file Supplementary.tex]

%% For double-blind review submission, w/o CCS and ACM Reference (max submission space)
\documentclass[sigconf,review,anonymous]{acmart}
\settopmatter{printfolios=true,printccs=false,printacmref=false}
 % For double-blind review submission, w/ CCS and ACM Reference
%\documentclass[sigplan,review,anonymous]{acmart}\settopmatter{printfolios=true}
%% For single-blind review submission, w/o CCS and ACM Reference (max submission space)
%\documentclass[sigplan,review]{acmart}\settopmatter{printfolios=true,printccs=false,printacmref=false}
%% For single-blind review submission, w/ CCS and ACM Reference
%\documentclass[sigplan,review]{acmart}\settopmatter{printfolios=true}
%% For final camera-ready submission, w/ required CCS and ACM Reference
%\documentclass[sigplan]{acmart}\settopmatter{}

\acmConference[ICSE 2020]{42nd International Conference on Software Engineering}{23--29 May, 2020}{Seoul, South Korea}

%% Conference information
%% Supplied to authors by publisher for camera-ready submission;
%% use defaults for review submission.
% \acmConference[PL'18]{ACM SIGPLAN Conference on Programming Languages}{January 01--03, 2018}{New York, NY, USA}
% \acmYear{2018}
% \acmISBN{} % \acmISBN{978-x-xxxx-xxxx-x/YY/MM}
% \acmDOI{} % \acmDOI{10.1145/nnnnnnn.nnnnnnn}
% \startPage{1}

%% Copyright information
%% Supplied to authors (based on authors' rights management selection;
%% see authors.acm.org) by publisher for camera-ready submission;
%% use 'none' for review submission.
\setcopyright{none}
%\setcopyright{acmcopyright}
%\setcopyright{acmlicensed}
%\setcopyright{rightsretained}
%\copyrightyear{2018}           %% If different from \acmYear

%% Bibliography style
\bibliographystyle{ACM-Reference-Format}
%% Citation style
%\citestyle{acmauthoryear}  %% For author/year citations
%\citestyle{acmnumeric}     %% For numeric citations
%\setcitestyle{nosort}      %% With 'acmnumeric', to disable automatic
                            %% sorting of references within a single citation;
                            %% e.g., \cite{Smith99,Carpenter05,Baker12}
                            %% rendered as [14,5,2] rather than [2,5,14].
%\setcitesyle{nocompress}   %% With 'acmnumeric', to disable automatic
                            %% compression of sequential references within a
                            %% single citation;
                            %% e.g., \cite{Baker12,Baker14,Baker16}
                            %% rendered as [2,3,4] rather than [2-4].

%%%%%%%%%%%%%%%%%%%%%%%%%%%%%%%%%%%%%%%%%%%%%%%%%%%%%%%%%%%%%%%%%%%%%%
%% Note: Authors migrating a paper from traditional SIGPLAN
%% proceedings format to PACMPL format must update the
%% '\documentclass' and topmatter commands above; see
%% 'acmart-pacmpl-template.tex'.
%%%%%%%%%%%%%%%%%%%%%%%%%%%%%%%%%%%%%%%%%%%%%%%%%%%%%%%%%%%%%%%%%%%%%%

\input{macros}

\begin{document}

%% Title information
\title{\tool: A Framework for Testing \\
Autonomous Driving Systems}         %% [Short Title] is optional;
                                        %% when present, will be used in
                                        %% header instead of Full Title.
%\titlenote{Supplementary material}             %% \titlenote is optional;
                                        %% can be repeated if necessary;
                                        %% contents suppressed with 'anonymous'
\subtitle{Supplementary material}                     %% \subtitle is optional
%\subtitlenote{with subtitle note}       %% \subtitlenote is optional;
                                        %% can be repeated if necessary;
                                        %% contents suppressed with 'anonymous'

%% Author information
%% Contents and number of authors suppressed with 'anonymous'.
%% Each author should be introduced by \author, followed by
%% \authornote (optional), \orcid (optional), \affiliation, and
%% \email.
%% An author may have multiple affiliations and/or emails; repeat the
%% appropriate command.
%% Many elements are not rendered, but should be provided for metadata
%% extraction tools.

%% Author with single affiliation.
\author{First1 Last1}
\authornote{with author1 note}          %% \authornote is optional;
                                        %% can be repeated if necessary
\orcid{nnnn-nnnn-nnnn-nnnn}             %% \orcid is optional
\affiliation{
  \position{Position1}
  \department{Department1}              %% \department is recommended
  \institution{Institution1}            %% \institution is required
  \streetaddress{Street1 Address1}
  \city{City1}
  \state{State1}
  \postcode{Post-Code1}
  \country{Country1}                    %% \country is recommended
}
\email{first1.last1@inst1.edu}          %% \email is recommended

%% Author with two affiliations and emails.
\author{First2 Last2}
\authornote{with author2 note}          %% \authornote is optional;
                                        %% can be repeated if necessary
\orcid{nnnn-nnnn-nnnn-nnnn}             %% \orcid is optional
\affiliation{
  \position{Position2a}
  \department{Department2a}             %% \department is recommended
  \institution{Institution2a}           %% \institution is required
  \streetaddress{Street2a Address2a}
  \city{City2a}
  \state{State2a}
  \postcode{Post-Code2a}
  \country{Country2a}                   %% \country is recommended
}
\email{first2.last2@inst2a.com}         %% \email is recommended
\affiliation{
  \position{Position2b}
  \department{Department2b}             %% \department is recommended
  \institution{Institution2b}           %% \institution is required
  \streetaddress{Street3b Address2b}
  \city{City2b}
  \state{State2b}
  \postcode{Post-Code2b}
  \country{Country2b}                   %% \country is recommended
}
\email{first2.last2@inst2b.org}         %% \email is recommended

%% 2012 ACM Computing Classification System (CSS) concepts
%% Generate at 'http://dl.acm.org/ccs/ccs.cfm'.
\begin{CCSXML}
<ccs2012>
<concept>
<concept_id>10011007.10011006.10011008</concept_id>
<concept_desc>Software and its engineering~General programming languages</concept_desc>
<concept_significance>500</concept_significance>
</concept>
<concept>
<concept_id>10003456.10003457.10003521.10003525</concept_id>
<concept_desc>Social and professional topics~History of programming languages</concept_desc>
<concept_significance>300</concept_significance>
</concept>
</ccs2012>
\end{CCSXML}

\ccsdesc[500]{Software and its engineering~General programming languages}
\ccsdesc[300]{Social and professional topics~History of programming languages}
%% End of generated code

%% Keywords
%% comma separated list
% \keywords{keyword1, keyword2, keyword3}  %% \keywords are mandatory in final camera-ready submission

%% \maketitle
%% Note: \maketitle command must come after title commands, author
%% commands, abstract environment, Computing Classification System
%% environment and commands, and keywords command.

\maketitle

\input{Supplementary-text}

%% Acknowledgments
% \begin{acks}                            %% acks environment is optional
                                        %% contents suppressed with 'anonymous'
% \end{acks}

%% Bibliography
\bibliography{Bibliography}

%% Appendix
%\clearpage
%\appendix
%\input{appendix/appendix}

\end{document}
